# Supplementary material for: Non-uniformity is All You Need: Efficient and Timely Encrypted Traffic Classification With ECHO
Source: arXiv:2406.01852 source file (2024-07-09)
Supplement: Supplementary file 1 [file appendix.tex]

\section{Appendix?}
